# Supplementary material for: Spectra of Gurtin-Pipkin type of integro-differential equations and applications to waves in graded viscoelastic structures
Source: arXiv:2004.02828 source file (2020-07-01)
Supplement: Supplementary file 1 [file S4_additional.tex]

\section{Additional material for full paper}

\begin{itemize}
	\item What about the closure of rational, polynomial, and operator for Boltzmann?
	\item Relation in-between eigenvectors (all cases)
	\item What about the essential spectrum?
\end{itemize}
