# Supplementary material for: Spectra of Gurtin-Pipkin type of integro-differential equations and applications to waves in graded viscoelastic structures
Source: arXiv:2004.02828 source file (2020-07-01)
Supplement: Supplementary file 2 [file S5_additional.tex]

\section{Additional material for full paper}

\begin{itemize}
	\item What about the closure of rational, polynomial, and operator for Boltzmann?
	\item Relation in-between eigenvectors (all cases)
	\item What about the essential spectrum?
\end{itemize}
Vlasov, bla bla studied the point spectrum and solvability of $T(\lambda)u=h$ when $T_b$ is a positive multiple of $T_b$. The focus in thous papers are on deriving interesting results for general kernels under the assumption that the material properties are independent of space and the equations are dependent of one space variable. In particular, Erenkko and Ivanov studied the case $\Omega=(0,\pi)$, $T_a=-a\frac{d^2}{dx^2}$, $T_b=-\frac{d^2}{dx^2}$ and define the function
\[
	G_n(z))z^2+az^2-n^2K(z)
\] 
That the spectrum of () is in the paper defined as the union of all zeros of $G_n$, $n=1,2,\dots$. In our notation is this the point spectrum of $T$, since it coincides with the solutions of $T(\lambda)u=0$ with $u=\sum c_n\sin (nx)$.
